# Supplementary material for: Bayesian Bootstraps for Massive Data
Source: arXiv:1705.09998 ancillary file (2019-03-22)
Supplement: Supplementary file 1 [file Supplementary_material_Bayesian_Bootstraps_for_Massive_Data.pdf]

# Supplementary material: Bayesian Bootstraps for Massive Data

ANDRÉS F. BARRIENTOS, VÍCTOR PEÑA*

March 21, 2019

This document has 6 sections: the first provides theoretical results for the processes proposed in Sections 2.1, 2.2, and 2.3; the second has a figure which details the Monte Carlo algorithm for performing lossless inference for the class of functionals described in Section 2.3; the third contains a scheme for lossless simulation for the example in Section 2.3 in Chamberlain and Imbens (2003); the fourth part explains how to perform lossless inference for the Dirichlet-Multinomial process; the fifth includes a table with relative and absolute errors related to the linear regression coefficients estimated from the OPM-2011 dataset in Section 4.1; Finally, the sixth assesses the performance of the BLBB, SDBB, ANs, and AN approximating coefficients of a quantile regression fitted to the OPM-2011 dataset.

## 1 Theoretical results

In this section we provide asymptotic results for the processes proposed in Section 2 of the paper. The results provided for the BLBB and SDBB processes resemble Theorem 1 in Kleiner et al. (2014) and Theorem 1 in Sengupta et al. (2016), respectively. The results derived for the BLDP and SDDP process correspond to a variation of Theorem 3.1 in James (2008).

### Large sample properties for the BLBB

The following theorem characterizes approximation properties of the BLBB by exploiting asymptotic arguments from the theory of *weighted bootstrap empirical process* (see Section 3.6.2 of van der Vaart and Wellner, 1996).

**Theorem 1.** *Assume that $P_0$ is the true data generating mechanism. Suppose that $T$ is Hadamard differentiable at $P_0$ tangentially to some subspace, with $P_0$, $P_n^{\text{BB}}$ and $P_{j,b,n}^{\text{BLBB}}$ viewed as maps from some Donsker class $\mathcal{F}$ to $\mathbb{R}$ such that $\mathcal{F}_\delta$ is measurable for every $\delta > 0$, where $\mathcal{F}_\delta = \{f - g :$*

*Andrés F. Barrientos is Postdoctoral Associate, Department of Statistical Science, Duke University, Durham, NC 27708 (email: afb26@stat.duke.edu) and, Víctor Peña is Assistant Professor, Department of Information Systems and Statistics, Baruch College, New York, NY 10010.

*$f, g \in \mathcal{F}, \delta_{P_0}(f-g) < \delta\}$ and $\delta_{P_0}(f) = \{P_0(f - P_0 f)^2\}^{1/2}$. Additionally, assume that $\pi_{\phi_T}(\cdot|\mathcal{X}_n) \mapsto \xi\{\pi_{\phi_T}(\cdot|\mathcal{X}_n)\}$ and $\tilde{\pi}^{\text{BLBB}}_{\phi_T}(\cdot|\mathcal{X}_{j,b,n}) \mapsto \xi\{\tilde{\pi}^{\text{BLBB}}_{\phi_T}(\cdot|\mathcal{X}_{j,b,n})\}$ are continuous with respect to a metric that metrizes weak convergence. Then,*

$$s^{-1}\sum_{j=1}^{s} \xi\{\tilde{\pi}^{\text{BLBB}}_{\phi_T}(\cdot|\mathcal{X}_{j,b,n})\} - \xi\{\pi_{\phi_T}(\cdot|\mathcal{X}_n)\} \to 0, \text{ in } P_0\text{-probability,}$$

*as $n \to \infty$, $b \to \infty$, $n/b = \tilde{s}$, and for any fixed $\tilde{s}$ and $s$ with $s \le \tilde{s}$.*

*Proof.* We start noticing that $\mathbb{G}^{\text{BB}}_n := \sqrt{n}(P^{\text{BB}}_n - P_0)$ and $\mathbb{G}^{\text{BLBB}}_{j,b,n} := \sqrt{n}(P^{\text{BLBB}}_{j,b,n} - E[P^{\text{BLBB}}_{j,b,n}|\mathcal{X}_{j,b,n}])$ are $\mathcal{F}$-indexed empirical processes and belong to the class of *weighted bootstrap empirical process* defined in Section 3.6.2 of van der Vaart and Wellner (1996). Since $\mathcal{F}$ is a Donsker class and $\tilde{s}$ is fixed, $\mathbb{G}^{\text{BB}}_n$ and $\mathbb{G}^{\text{BLBB}}_{j,b,n}$ converges weakly, in $P_0$-probability, to a $P_0$-Browian bridge process $\mathbb{G}$ as $n \to \infty$. This convergence is ensured by Theorem 3.6.13 of van der Vaart and Wellner (1996). Thus, given that $T$ is Hadamard differentiable at $P_0$, and by Theorem 3.9.11 of van der Vaart and Wellner (1996), $\phi_T(P^{\text{BB}}_n, \mathbb{P}_n)$ and $\phi_T(P^{\text{BLBB}}_{j,b,n}, \mathbb{P}_{j,b,n})$ converges weakly to $T'_{P_0}(\mathbb{G})$, in $P_0$-probability, where $T'_{P_0}$ is the Hadamard derivative of $T$ at $P_0$. The proof is completed by using the continuity assumed for $\xi$ which implies that $|\xi\{\tilde{\pi}^{\text{BLBB}}_{\phi_T}(\cdot|\mathcal{X}_{j,b,n})\} - \xi\{\pi_{\phi_T}(\cdot|\mathcal{X}_n)\}| \to 0$, in $P_0$ probability, as $n \to \infty$. □

## Large sample properties for the SDBB

The following theorem provides conditions that ensure that the processes $\sqrt{n}(P^{\text{SDBB}}_{b,n} - E[P^{\text{SDBB}}_{b,n}|\mathcal{X}_n, R])$ and $\sqrt{n}(P^{\text{BB}}_n - E[P^{\text{BB}}_n|\mathcal{X}_n])$ converge to the same distribution. After proving this theorem, we explain conditions that $\phi_T$ and $\xi$ must meet so that $\pi^{\text{SDBB}}_{\phi_T}(\cdot|\mathcal{X}_n)$ can asymptotically approximate $\xi(\pi_{\phi_T}(\cdot|\mathcal{X}_n))$.

**Theorem 2.** *Assume that $P_0$ is the true data generating mechanism. Assume that $\mathcal{F}$ is a Donsker class for $P_0$ and additionally $\mathcal{F}_\delta = \{f - g : f, g \in \mathcal{F}, P(f-g)^2 \le \delta\}$ is measurable in the sense discussed in Giné and Zinn (1984) for each $\delta > 0$. Then we have for $min(n, b) \to \infty$*

$$\mathbb{G}^{\text{SDBB}}_{n,b} = \sqrt{n}\sum_{i=1}^{b}(\tilde{W}_i - 1/b) f(X_{R_i}) \underset{\tilde{W},R}{\overset{P_0}{\rightsquigarrow}} \mathbb{G}$$

*in $\ell^\infty(\mathcal{F})$, where $\mathbb{G}$ denotes a centered Gaussian process with covariance $E[\mathbb{G}(f), \mathbb{G}(g)] = cov(\mathbb{G}(f), \mathbb{G}(g))$, and $\underset{\tilde{W},R}{\overset{P_0}{\rightsquigarrow}}$ denotes conditional weak convergence in the sense described in Kosorok (2008), Section 2.2.3.*

*Proof.* We begin this proof by defining the map

$$f \mapsto (Z_n(R, X, \tilde{W}))(f) := \sqrt{n}\sum_{i=1}^{b}(\tilde{W}_i - 1/b) f(X_{R_i}),\ f \in \mathcal{F},$$

where $(Z_n(R, X, \tilde{W}))(\cdot)$ can be viewed as a $\ell^\infty(\mathcal{F})$-valued stochastic process, $\tilde{W} = (\tilde{W}_i, \dots, \tilde{W}_n)$, and $R = (R_1, \dots, R_b)$. Thus, under this new mapping, proving that $\mathbb{G}_{n,b}^{\text{SDBB}} \underset{\tilde{W},R}{\overset{P_0}{\rightsquigarrow}} \mathbb{G}$ is equivalent to showing that (see Section 2.2.3 of Kosorok, 2008)

(i)

$$\sup_{h \in \mathrm{BL}_1} \left| E\left[ h(Z_n(R, X, \tilde{W})) | \mathcal{X}_n \right] - E\left[ h(\mathbb{G}) \right] \right| \xrightarrow{P_0} 0 \text{ and,}$$

(ii) for all $h \in \mathrm{BL}_1$,

$$E\left[ h(Z_n(R, X, \tilde{W}))^* | \mathcal{X}_n \right] - E\left[ h(Z_n(R, X, \tilde{W}))_* | \mathcal{X}_n \right] \xrightarrow{P_0} 0,$$

where $\mathrm{BL}_1$ denotes the set of Lipschitz continuous functions $h : \ell^\infty(\mathcal{F}) \to \mathbb{R}$ with Lipschitz constant 1 that are additionally uniformly bounded by 1. Here, we use the notation $f^*$ and $f_*$ to denote the smallest measurable majorant and greatest measurable minorant, respectively. Similarly, we use the notation $g(R, x, \tilde{W})^{*,R,\tilde{W}}$ and $g(R, X, \tilde{W})_{*,R,\tilde{W}}$ to denote the smallest measurable majorant and greatest measurable minorant of the map $(r, \tilde{w}) \mapsto g(r, x, \tilde{w})$ with $x$ being held fixed. We now proceed to prove (i) and (ii) by borrowing the inequalities derived in proof of Theorem 1 of Sengupta et al. (2016). Thus, for (i) and (ii), we have that

$$\begin{aligned} & E^*\left[ \sup_{h \in \mathrm{BL}_1} \left| E\left[ h(Z_n(R, X, \tilde{W})) | \mathcal{X}_n \right] - E\left[ h(\mathbb{G}) \right] \right| \right] \\ \leq \quad & E^*\left[ \sup_{h \in \mathrm{BL}_1} \left| E\left[ h(Z_n(\mathrm{id}, X, \tilde{W})) | \mathcal{X}_n \right] - E\left[ h(\mathbb{G}) \right] \right| \right] \end{aligned}$$

and

$$\begin{aligned} & E\left[ h(Z_n(R, X, \tilde{W}))^* | \mathcal{X}_n \right] - E\left[ h(Z_n(R, X, \tilde{W}))_* | \mathcal{X}_n \right] \\ \leq \quad & E\left[ h(Z_n(\mathrm{id}, X, \tilde{W}))^{*,R,W} \right] - E\left[ h(Z_n(\mathrm{id}, X, \tilde{W}))_{*,R,W} \right], \end{aligned}$$

respectively. Here, $E^*$ denotes outer expectation and $\mathrm{id} := (1, \dots, b)$. Finally, by Theorem 3.9.11 of van der Vaart and Wellner (1996) and dominated convergence, we have that

$$E^*\left[ \sup_{h \in \mathrm{BL}_1} \left| E\left[ h(Z_n(\mathrm{id}, X, \tilde{W})) | \mathcal{X}_n \right] - E\left[ h(\mathbb{G}) \right] \right| \right] \to 0$$

and

$$E\left[ h(Z_n(\mathrm{id}, X, \tilde{W}))^{*,R,W} \right] - E\left[ h(Z_n(\mathrm{id}, X, \tilde{W}))_{*,R,W} \right] \to 0.$$

This completes the proof of this theorem. □

Notice that we need to identify the process $\mathbb{G}_{n,b}^{\text{SDBB}}$ in above theorem with the process $\sqrt{n}(P_{b,n}^{\text{SDBB}} - E[P_{b,n}^{\text{SDBB}} | \mathcal{X}_n])$ and that $\mathbb{G}$ is the limiting distribution of $\sqrt{n}(P_n^{\text{BB}} - E[P_n^{\text{BB}} | \mathcal{X}_n)]$. Thus, if we assume the functional $\phi_T$ satisfies the condition (H) of Sengupta et al. (2016), we can use the functional delta method to prove that $\sqrt{n}(T(P_{b,n}^{\text{SDBB}}) - T(E[P_{b,n}^{\text{SDBB}} | \mathcal{X}_n]))$ and $\sqrt{n}(T(P_n^{\text{BB}}) - T(E[P_n^{\text{BB}} | \mathcal{X}_n]))$ have the same limiting distribution. Finally, if we also assume that $\pi_{\phi_T}(\cdot | \mathcal{X}_n) \mapsto \xi(\pi_{\phi_T}(\cdot | \mathcal{X}_n))$ is continuous in the space of $\pi_{\phi_T}(\cdot | \mathcal{X}_n)$ with respect to a metric that metrizes weak convergence, then $\xi\{\pi_{\phi_T}^{\text{SDBB}}(\cdot | \mathcal{X}_n)\} - \xi\{\pi_{\phi_T}(\cdot | \mathcal{X}_n)\}$ converges to zero.

## Large sample properties for the BLDP and SDDP

Theorem 3.1 in James (2008) provides conditions that ensure that $\sqrt{n}(P_n^{\text{DP}} - E[P_n^{\text{DP}}|\mathcal{X}_{b,n}])$ converges weakly conditionally on the data to a $P_0$-Browian bridge process $\mathbb{G}$. The following result, which is a variation of Theorem 3.1 in James (2008), shows that $\sqrt{n}(P_{j,b,n}^{\text{BLDP}} - E[P_{j,b,n}^{\text{BLDP}}|\mathcal{X}_{j,b,n}])$ and $\sqrt{n}(P_{b,n}^{\text{SDDP}} - E[P_{b,n}^{\text{SDDP}}|\mathcal{X}_n, R])$ have the same limit distribution as $\sqrt{n}(P_n^{\text{DP}} - E[P_n^{\text{DP}}|\mathcal{X}_{b,n}])$.

**Theorem 3.** *Assume that $P_0$ is the true data generating mechanism and continuous. Let $\mathcal{F}$ be a Vapnik-Chervonenkis graphclass subclass of $L_2(P_0)$ and $L_2(H)$ with envelop $F$ such that $P_0(F^2) < \infty$ and $H(F^2) < \infty$. Then, conditional on the data,*

*i)* $\sqrt{n}(P_{j,b,n}^{\text{BLDP}} - E[P_{j,b,n}^{\text{BLDP}}|\mathcal{X}_{j,b,n}])$ *converges weakly to $\mathbb{G}$ in $\ell^\infty(\mathcal{F})$ and in $P_0$-probability as $n \to \infty$, $b \to \infty$, $n/b = \tilde{s}$, and for any fixed $\tilde{s}$.*

*ii)* $\sqrt{n}(P_{b,n}^{\text{SDDP}} - E[P_{b,n}^{\text{SDDP}}|\mathcal{X}_n, R])$ *converges weakly to $\mathbb{G}$ in $\ell^\infty(\mathcal{F})$ and in $P_0$-probability as $min(n, b) \to \infty$.*

*Proof.* Borrowing the trick used in proof of Theorem 3.1 in James (2008), we first note that $\sqrt{n}(P_{j,b,n}^{\text{BLDP}} - E[P_{j,b,n}^{\text{BLDP}}|\mathcal{X}_{j,b,n}])$ and $\sqrt{n}(P_{b,n}^{\text{SDDP}} - E[P_{b,n}^{\text{SDDP}}|\mathcal{X}_n, R])$ are equivalent to

$$(1 - R_n)\mathbb{G}_{j,b,n}^{\text{BLBB}} + \sqrt{n}\left(R_n - \frac{\alpha}{\alpha + n}\right)(H - \mathbb{P}_{j,b,n}) + R_n\sqrt{n}(P^{\text{DP}} - H), \text{ and}$$

$$(1 - R_n)\mathbb{G}_{n,b}^{\text{SDBB}} + \sqrt{n}\left(R_n - \frac{\alpha}{\alpha + n}\right)(H - b^{-1}\sum_{i=1}^{b}\delta_{X_{R_i}}) + R_n\sqrt{n}(P^{\text{DP}} - H),$$

respectively. Since $R_n$, $\sqrt{n}(R_n - \alpha/(\alpha + n))$ and $\sqrt{n}R_n$ converge to zero, then $\sqrt{n}(P_{j,b,n}^{\text{BLBB}} - E[P_{j,b,n}^{\text{BLBB}}|\mathcal{X}_{j,b,n}])$ and $\sqrt{n}(P_{b,n}^{\text{SDDP}} - E[P_{b,n}^{\text{SDDP}}|\mathcal{X}_n, R])$ has the same limit distribution as $\mathbb{G}_{j,b,n}^{\text{BLBB}}$ and $\mathbb{G}_{n,b}^{\text{SDBB}}$. Given that $\mathcal{F}$ is also a Donsker class, we have that $\mathbb{G}_{j,b,n}^{\text{BLBB}}$ and $\mathbb{G}_{n,b}^{\text{SDBB}}$ converge weakly to $\mathbb{G}$ in $P_0$-probability (see proof of Theorems 1 and 2). This completes the proof of this theorem. □

## 2 Algorithm for lossless inference

**Input:** Data $\mathcal{X}_n = \{X_1, \dots, X_n\}$

$\phi, g, \rho$: functionals of interest  $\xi$: posterior summary of interest

$b$: subset size

**Output:** Monte Carlo approximation of $\xi\left(\pi_\phi\left(\cdot|\mathcal{X}_n\right)\right)$

Let $\mathcal{I}_{1,b}, \dots, \mathcal{I}_{n/b,b}$ be a partition of the set $\{1, \dots, n\}$, where

$\mathcal{I}_{j,b} = \{1 + (j-1)b, \dots, jb\}$

```
for j ← 1 to n/b do
    for l ← 1 to r do
        sample (z_1, ..., z_b) ~ Gamma(1, 1)
        t_{j,1}^{(l)} ← Σ_{i∈I_{j,b}} z_i ρ_1(X_i)
        ⋮
        t_{j,k}^{(l)} ← Σ_{i∈I_{j,b}} z_i ρ_k(X_i)
        s_j^{(l)} ← Σ_{i∈I_{j,b}} z_i
    end
end
for l ← 1 to r do
    q_1^{(l)} ← (Σ_{j=1}^{n/b} s_j^{(l)})^{-1} Σ_{j=1}^{n/b} s_j t_{j,1}^{(l)}
    ⋮
    q_k^{(l)} ← (Σ_{j=1}^{n/b} s_j^{(l)})^{-1} Σ_{j=1}^{n/b} s_j t_{j,k}^{(l)}
    Q^{(l)} ← g(q_1^{(l)}, ..., q_k^{(l)})
end
π_φ(·|X_n) ← r^{-1} Σ_{l=1}^{r} δ_{Q^{(l)}}(·)
return ξ(π_φ(·|X_n))
```

**Figure 1.** Monte Carlo algorithm for lossless inference for functionals in the class described in Section 2.3

# 3 Lossless Inference for Section 2. in Chamberlain and Imbens (2003)

Let $y_n$ be the outcome, $T_n$ the treatment, $z_n$ the instrument for individuals $n \in \{1, 2, \ldots, N\}$. We have independent and identically distributed $(y_n, z_n, T_n)|P \sim P$ and let $P$ given the data be distributed as the Bayesian bootstrap. For notational convenience, we use the vectorized notation

$$\begin{aligned}
Y &= (y_1\, y_2 \ldots y_N)^\top \\
T &= (t_1\, t_2 \ldots t_n)^\top \\
Z &= (z_1\, z_2 \ldots, z_n)^\top \\
1_n &= (1\, 1 \overset{(n)}{\ldots} 1)^\top \\
X &= [1_n\, T]
\end{aligned}$$

Following Chamberlain and Imbens (2003), the parameter of interest is the two-dimensional vector $\beta$ that solves

$$\begin{aligned}
\mathbb{E}_P[Y - X\beta] &= 0 \\
\mathbb{E}_P[Z'(Y - X\beta)] &= 0.
\end{aligned}$$

The uncertainty in $P$ propagates to $\beta$, so it is a random variable.

One can sample from the posterior of $\beta$ as follows:

1. Sample $(V_n)_{n=1}^N$, where $V_n \overset{\text{iid}}{\sim} \text{Exp}(1)$.
2. Using the algorithm described in Section 2.3 of our article, find

$$\begin{aligned}
A = \sum_{n=1}^N V_n,\ B = \sum_{n=1}^N V_n T_n,\ C = \sum_{n=1}^N V_n y_n \\
D = \sum_{n=1}^N V_n z_n,\ E = \sum_{n=1}^N V_n y_n z_n,\ F = \sum_{n=1}^N V_n T_n z_n.
\end{aligned}$$

3. Find $\beta = (\beta_0,\, \beta_1)'$ as

$$\beta_1 = \frac{F - DBC/A}{E - DB/A},\ \ \beta_0 = (C - B\beta_1)/A.$$

4. Repeat 1-3 as many times as desired.

# 4 Lossless inference for the Dirichlet-Multinomial process

The Dirichlet process can be approximated by the Dirichlet-multinomial process, which is finite-dimensional. This model has been known and studied for decades; for instance, see Kingman (1975) and Pitman (1995). The results that are most relevant to our work can be found in Ishwaran and Zarepour (2002) and Muliere and Secchi (1996). The former shows weak convergence of $H$-integrable functionals of the Dirichlet-multinomial process to the Dirichlet process, while the latter shows weak convergence for quantiles. Section 4 in Ishwaran and Zarepour (2002) contains a thorough study of relevant properties of this approximation, which we do not reproduce here for brevity. The model is defined as follows:

$$\begin{aligned}\tilde{P}_n^{\text{DP}}(\cdot) &= \sum_{k=1}^{K} W_k\, \delta_{A_k}(\cdot)\\(W_k)_{k=1}^{K} &\sim \text{Dirichlet}\left(\frac{\alpha+n}{K}, \frac{\alpha+n}{K}, \dots, \frac{\alpha+n}{K}\right)\\A_i &\sim \frac{\alpha}{\alpha+n}H + \frac{n}{\alpha+n}\mathbb{P}_n.\end{aligned}$$

If $K = n$ and $n$ is large, the model behaves like the Bayesian bootstrap. In particular, as $n$ tends to infinity, the distribution of the weights converges weakly to the Dirichlet$(1, 1, \dots, 1)$, and the distribution of the $A_i$ converges weakly to the empirical probability measure.

A positive aspect of the Dirichlet-multinomial process is that one can perform "lossless inference" (in the sense that no further approximations are needed) for the class of functionals defined in Section 2.3 of the main text: the Dirichlet weights can be decomposed as a function of $Z_i \sim \text{Gamma}((\alpha+n)/K, 1)$ random variables and the algorithm described in Figure 3 of the main text can be adapted in an obvious manner. In this case, the theoretical guarantees in Muliere and Secchi (1996) and Ishwaran and Zarepour (2002) apply directly.

## 5 Linear regression: table of relative and absolute errors, OPM-2011 dataset

Table 1 contains average relative and absolute errors of approximate posterior summaries for $\boldsymbol{\beta}^{\text{BB}}_{\text{lm},n}$, OMP-2011 dataset. Section 4.1 of the manuscript provides a discussion of the values in this table.

**Table 1.** Average relative and absolute errors of approximate posterior summaries for $\boldsymbol{\beta}^{\text{BB}}_{\text{lm},n}$, OMP-2011 dataset. The average errors are computed over all regression coefficients. Relative errors are reported for CIL and SD; absolute errors are reported for Mean. CIL and SD stand for credible interval length and posterior standard deviation.

| n | Summary | $\gamma$ | BLBB | SDBB | ANS | AN |
|---|---|---|---|---|---|---|
| 50,000 | CIL | .6 | .037 | .030 | .053 | .047 |
| | | .7 | .038 | .031 | .048 | .047 |
| | | .8 | .033 | .033 | .047 | .047 |
| | SD | .6 | .017 | .021 | .041 | .036 |
| | | .7 | .019 | .017 | .038 | .036 |
| | | .8 | .020 | .017 | .037 | .036 |
| | Mean | .6 | <.001 | .001 | <.001 | <.001 |
| | | .7 | <.001 | .001 | <.001 | <.001 |
| | | .8 | <.001 | <.001 | <.001 | <.001 |
| 200,000 | CIL | .6 | .034 | .037 | .038 | .036 |
| | | .7 | .029 | .042 | .036 | .036 |
| | | .8 | .033 | .035 | .036 | .036 |
| | SD | .6 | .023 | .030 | .036 | .034 |
| | | .7 | .030 | .041 | .035 | .034 |
| | | .8 | .030 | .044 | .035 | .034 |
| | Mean | .6 | <.001 | .001 | <.001 | <.001 |
| | | .7 | <.001 | .001 | <.001 | <.001 |
| | | .8 | <.001 | <.001 | <.001 | <.001 |

# 6 Quantile regression: analysis of OPM-2011 dataset

In this section, we compare the BLBB, the SDBB, and the asymptotic methods (ANS and AN) in estimating $\tau$-quantile regression coefficients (Chamberlain and Imbens, 2003)

$$\boldsymbol{\beta}^{\text{BB}}_{\tau,n} = (\beta^{\text{BB}}_{0,\tau,n}, \ldots, \beta^{\text{BB}}_{p,\tau,n}) = \underset{\boldsymbol{\beta} \in \mathbb{R}^{p+1}}{\arg\min} \sum_{i=1}^{n} W_i c_\tau(Y_i - U_i^\top \boldsymbol{\beta}),$$

where $c_\tau(t) = |t| \left[(1-\tau)\mathbb{I}_{(-\infty,0)}(t) + \tau\mathbb{I}_{[0,\infty)}(t)\right.$ and, $\mathbb{I}_A(t) = 1$ if $t \in A$ and $\mathbb{I}_A(t) = 0$ otherwise. Here, we set $n =$200,000 and $\tau \in \{0.5, 0.25, 0.1\}$. Quantile regression is of special interest in this application because the social scientists who provided the data want to determine whether the effect of the predictors (race, education, sex, etc.) changes for different income levels (quantiles). For example, the effect of higher education might be lower for high income families than for lower income families (i.e. higher education is a strong factor for upward social mobility). Our implementation in R uses the method `fn` of the function `rq` in library `quantreg` (Koenker, 2017).

Table 2 presents the relative and absolute errors associated with $\boldsymbol{\beta}^{\text{BB}}_{\tau,n}$. The approximations are better for larger $\gamma$ and values of $\tau$ that are not extreme (near zero). The relative errors of the BLBB are smaller than the errors of the SDBB, and their biases (absolute error) are relatively similar and small. In general, the bias of the BLBB will be reduced when all the subsets in the partition can be processed and when the partition does not have "pathological" subsets. Regarding the asymptotic competitors, the relative errors of ANS and AN are almost always smaller than the errors of the BLBB and SDBB when $\gamma = 0.6,\ 0.7$. However, when $\gamma = 0.8$, the BLBB and ANS have similar performance. For this reason, we recommend using $\gamma$ as large as possible when using the BLBB. The ANS method has proved to be a strong competitor in this context, and further work is needed to identify the class of functionals for which this method should be preferred.

Figure 2 displays credible intervals for $(\beta^{\text{BB}}_{1,\tau,n}, \ldots, \beta^{\text{BB}}_{4,\tau,n})$. The coefficients are associated with different races, and estimating them well is of special interest in this application. The most problematic coefficient is $\beta^{\text{BB}}_{1,\tau,n}$ (represented as $\beta_1$ in the figure), which is associated with a category with small observed frequency (2%). This issue also arises in mixed-effects regression (see Section 4.1 of the manuscript for a more detailed discussion). Figure 2 shows that the BLBB and ANS perform well in approximating credible intervals regardless of the value of $\gamma$. On the other hand, the SDBB only approximates credible intervals well whenever $\gamma = 0.8$; for $\gamma = 0.6,\ 0.7$, the SDBB outputs considerably wider intervals than needed.

Now, we give an argument as to why the SDBB overestimates uncertainty. In the SDBB, each random subset is associated with a rescaled BB (with weights distributed as Dirichlet$(n/b, n/b, \ldots, n/b)$). In each iteration, the SDBB selects a subset and takes a sample of size 1 from the distribution of the functional of interest (that stems out of the rescaled bootstrap), so the SDBB will be accurate if these distributions are similar across random subsets. This occurs with linear, mixed-effects, and logistic regression, so we did not experience this issue there. However, in quantile regression, the distributions are not always centered at 0 (although their variability is roughly the same). As a result, the SDBB gives rise to longer

intervals than needed (in Section 5 of the manuscript we provide practical guidelines to prevent this issue). In contrast, the BLBB picks subsets, finds their variability, and combines them. Since the variabilities of the subsets are similar, the BLBB can quantify the overall uncertainty correctly.

**Table 2.** Average relative and absolute errors of approximate posterior summaries for $\beta^{\text{BB}}_{\tau,n}$, OMP-2011 dataset. The average errors are computed over all regression coefficients. Relative errors are reported for CIL and SD; absolute errors are reported for Mean. CIL and SD stand for credible interval length and posterior standard deviation.

| $\tau$ | Summary | $\gamma$ | BLBB | SDBB | ANS | AN |
|---|---|---|---|---|---|---|
| .50 | CIL | .6 | .129 | .726 | .110 | .091 |
| | | .7 | .091 | .202 | .112 | .091 |
| | | .8 | .112 | .077 | .107 | .091 |
| | SD | .6 | .246 | .523 | .127 | .101 |
| | | .7 | .072 | .113 | .121 | .101 |
| | | .8 | .089 | .070 | .121 | .101 |
| | Mean | .6 | .001 | .001 | .001 | <.001 |
| | | .7 | .001 | .001 | .001 | <.001 |
| | | .8 | <.001 | <.001 | .001 | <.001 |
| .25 | CIL | .6 | .279 | .889 | .109 | .078 |
| | | .7 | .175 | .438 | .111 | .078 |
| | | .8 | .093 | .182 | .106 | .078 |
| | SD | .6 | .420 | .736 | .108 | .077 |
| | | .7 | .238 | .341 | .110 | .077 |
| | | .8 | .128 | .147 | .099 | .077 |
| | Mean | .6 | .002 | .002 | .002 | <.001 |
| | | .7 | .001 | .001 | .001 | <.001 |
| | | .8 | .001 | <.001 | .001 | <.001 |
| .10 | CIL | .6 | .291 | 1.113 | .082 | .047 |
| | | .7 | .105 | .463 | .068 | .047 |
| | | .8 | .082 | .198 | .070 | .047 |
| | SD | .6 | .476 | 1.002 | .082 | .056 |
| | | .7 | .155 | .312 | .063 | .056 |
| | | .8 | .083 | .144 | .065 | .056 |
| | Mean | .6 | .002 | .002 | .002 | .001 |
| | | .7 | .001 | .002 | .001 | .001 |
| | | .8 | .001 | .001 | .001 | .001 |

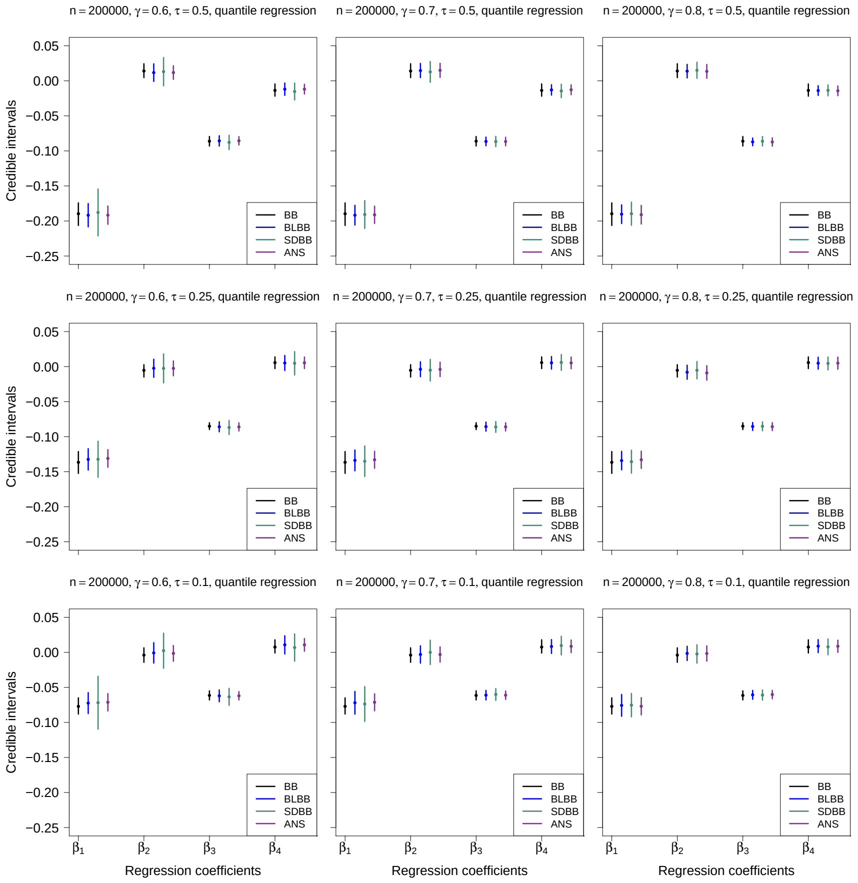


**Figure 2.** Credible intervals for quantile regression coefficients, $n$ =200,000, $\tau \in \{0.5, 0.25, 0.1\}$, and $\gamma \in \{0.6, 0.7, 0.8\}$. The displayed intervals are associated with the levels of the predictor race, OPM-2011 datasets.

# References


Chamberlain, G. and Imbens, G. W. (2003). Nonparametric applications of Bayesian inference. *Journal of Business & Economic Statistics*, 21(1):12–18.

Giné, E. and Zinn, J. (1984). Some limit theorems for empirical processes. *The Annals of Probability*, 12(4):929–998. With discussion.

Ishwaran, H. and Zarepour, M. (2002). Exact and approximate sum representations for the Dirichlet process. *Canadian Journal of Statistics*, 30(2):269–283.

James, L. F. (2008). Large sample asymptotics for the two-parameter Poisson–Dirichlet process. In *Pushing the limits of contemporary statistics: contributions in honor of Jayanta K. Ghosh*, pages 187–199. Institute of Mathematical Statistics.

Kingman, J. F. (1975). Random discrete distributions. *Journal of the Royal Statistical Society. Series B (Methodological)*, pages 1–22.

Kleiner, A., Talwalkar, A., Sarkar, P., and Jordan, M. I. (2014). A scalable bootstrap for massive data. *Journal of the Royal Statistical Society. Series B. Statistical Methodology*, 76(4):795–816.

Koenker, R. (2017). quantreg: Quantile regression. R package version 5.33.

Kosorok, M. R. (2008). *Introduction to empirical processes and semiparametric inference*. Springer Series in Statistics. Springer, New York.

Muliere, P. and Secchi, P. (1996). Bayesian nonparametric predictive inference and bootstrap techniques. *Annals of the Institute of Statistical Mathematics*, 48(4):663–673.

Pitman, J. (1995). Exchangeable and partially exchangeable random partitions. *Probability Theory and Related Fields*, 102:145–158.

Sengupta, S., Volgushev, S., and Shao, X. (2016). A subsampled double bootstrap for massive data. *Journal of the American Statistical Association*, 111(515):1222–1232.

van der Vaart, A. W. and Wellner, J. A. (1996). *Weak convergence and empirical processes*. Springer Series in Statistics. Springer-Verlag, New York. With applications to statistics.
